# Supplementary material for: Mining Functional Modules by Multiview-NMF of Phenome-Genome Association
Source: arXiv:1705.03998 source file (2017-05-11)
Supplement: Supplementary file 1 [file SI_11_25.pdf]

# Consistent Multiple Nonnegative Matrix Factorization with Hierarchical Information for Gene Functional Modules Mining

## Supporting Information (SI)

Files in this Data Supplement:

- SI Data Summary
- SI Measurement Definition
- SI Parameter Tuning

### SI Data Summary

The details of data used in our experiments have been summarized in Table 1.

### SI Measurement Definition

In our paper, we evaluate the gene clustering results with five external criteria. These criteria include $F_1$, *Precision*, *Recall*, *Jaccard Index* and *Rand Index*.

We use $n$ to denote the total gene number, all genes can be denoted as $S = \{O_1, ..., O_n\}$, we use gene pathways $X = \{X_1, ..., X_r\}$ as the ground-truth partition of genes, and use clustering result $Y = \{Y_1, ..., Y_s\}$ as prediction partitions, then define the following notations:

- TP, the number of pairs of elements in $S$ that are in the same set in $X$ and in the same set in $Y$
- TN, the number of pairs of elements in $S$ that are in different sets in $X$ and in different sets in $Y$

Table 1: Data Description

| Dataset | Relations (A-B) | Number of A | Number of B | Number of (A-B) |
|---|---|---|---|---|
| mouse | Gene-Phenotype(parent) | 1350 | 2557 | 6889 |
| | Gene-Phenotype(child) | 1350 | 3414 | 8635 |
| | Parent-child Phenotype Relation | 2557 | 3414 | 2995 |
| | PPI (Gene-Gene) (Feb. 2016) | 6234 | 6234 | 14715 |
| | PPI (Gene-Gene) (Sep. 2016) | 6234 | 6234 | 26190 |
| | Genes-Pathway (Feb. 2016) | 7753 | 292 | - |
| | Genes-Pathway (Sep. 2016) | 7882 | 292 | - |
| human | Gene-Phenotype(parent) | 3280 | 2241 | 23532 |
| | Gene-Phenotype(child) | 3280 | 3707 | 30397 |
| | Parent-child Phenotype Relation | 2241 | 3707 | 2702 |
| | PPI (Gene-Gene) (Feb. 2016) | 20585 | 20585 | 261847 |
| | PPI (Gene-Gene) (Sep. 2016) | 20585 | 20585 | 483838 |
| | Genes-Pathway (Feb. 2016) | 6989 | 296 | - |
| | Genes-Pathway (Sep. 2016) | 7087 | 296 | - |

Number of (A-B): the association number between A and B.

- FN, the number of pairs of elements in $S$ that are in the same set in $X$ and in different sets in $Y$
- FP, the number of pairs of elements in $S$ that are in different sets in $X$ and in the same set in $Y$

Now we can define the evaluation measures as below:

$$F_1\ measure = \frac{2PR}{P+R} \quad (P = \frac{TP}{TP+FP}, R = \frac{TP}{TP+FN})$$

$$Jaccard\ Index = \frac{TP}{TP+FP+FN}$$

$$Rand\ Index = \frac{TP+TN}{TP+FP+FN+TN}$$

## SI Parameter Tuning

The details of parameter tuning of CMNMF on mouse PPI network, human KEGG pathways and human PPI network are presented in this part.

We search $\alpha$ in {0.001, 0.01, 0.1, 1, 10, 100, 1000} and $\beta$ in {0.001, 0.01, 0.1, 1, 10, 100, 1000} for CMNMF, the darker the color, the higher the $F_1$ scores under the corresponding $\alpha$ and $\beta$ combinations. In this experiment, $\alpha = 1000$ and $\beta = 0.01$ are chosen as the best parameters while mouse PPI network is used as validation set (See Fig. 1). Fig. 2(a) shows $F_1$ scores while human KEGG pathways are used as validation set, it achieves the best performance when $\alpha = 1000$ and $\beta = 1000$. Fig. 2(b) shows $F_1$ scores while human PPI network is used as validation set, $\alpha = 1$ and $\beta = 0.1$ are the best parameters.

The HMF and ColNMF models contain one hyper-parameters, which balances the weight given to the hierarchical relation between parent ontologies and child ontologies. The parameter in HMF and ColNMF is selected among {0.001, 0.01, 0.1, 1, 10, 100, 1000}. For AHC and K-means, they are unsupervised clustering methods, in order to have a relatively fair comparison with other methods, we introduce additional pairwise constraints AHC [1] and pairwise constraints K-means [2], the old versions of KEGG pathways (Feb. 2016) and PPI network (Feb. 2016) are used as pairwise constraint validation set to help get clustering results.

# References


[1] Miyamoto, S., Terami, A.: Semi-supervised agglomerative hierarchical clustering algorithms with pairwise constraints. 2010 IEEE World Congress on Computational Intelligence, WCCI 2010, 2–7 (2010)

[2] Wagstaff, K., Cardie, C., Rogers, S., Schroedl, S.: Constrained K-means Clustering with Background Knowledge. International Conference on Machine Learning, 577–584 (2001)

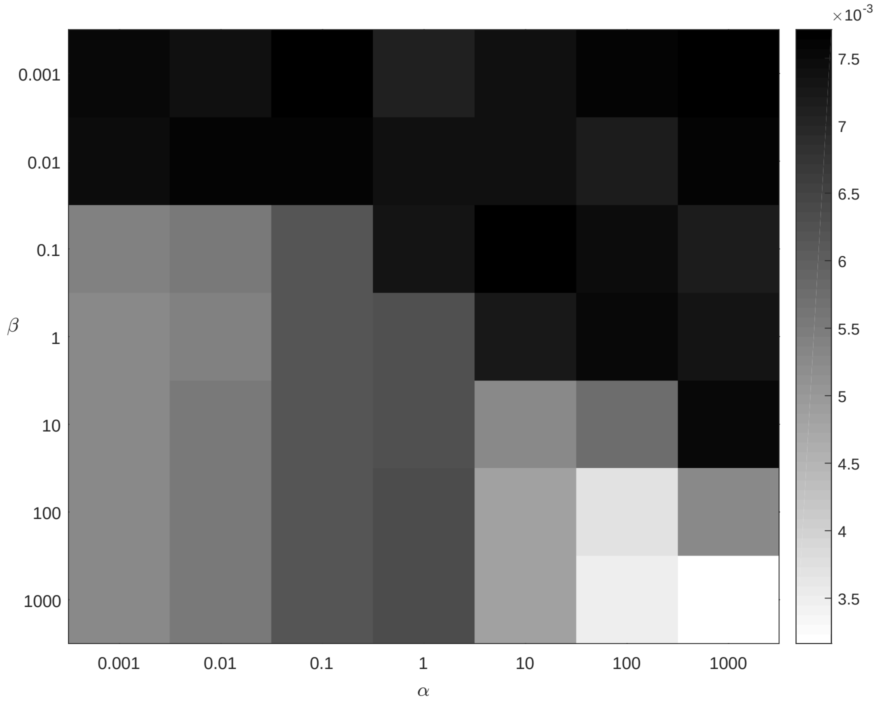


Figure 1: Mouse PPI network was used as validation set

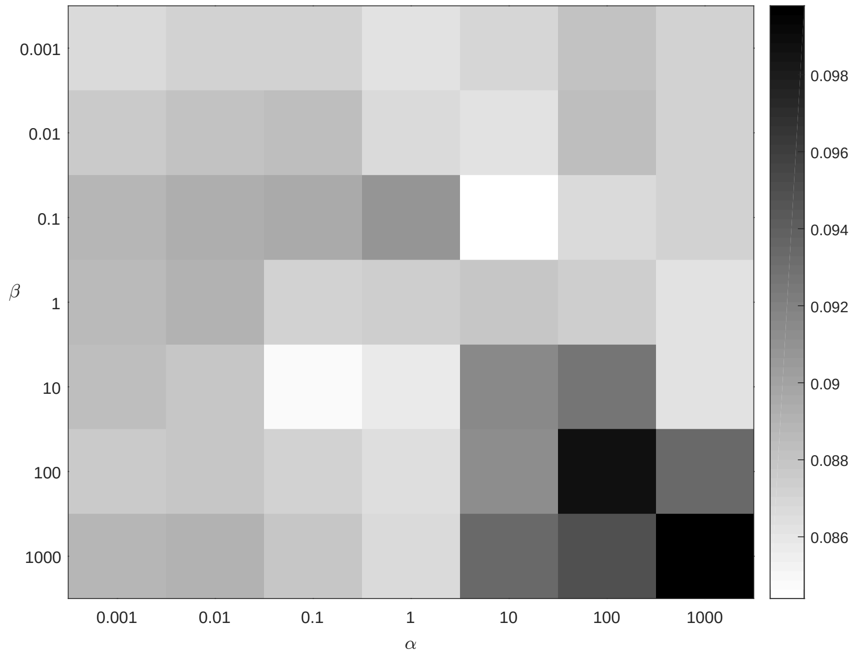


(a) Human KEGG Pathways were used as validation set

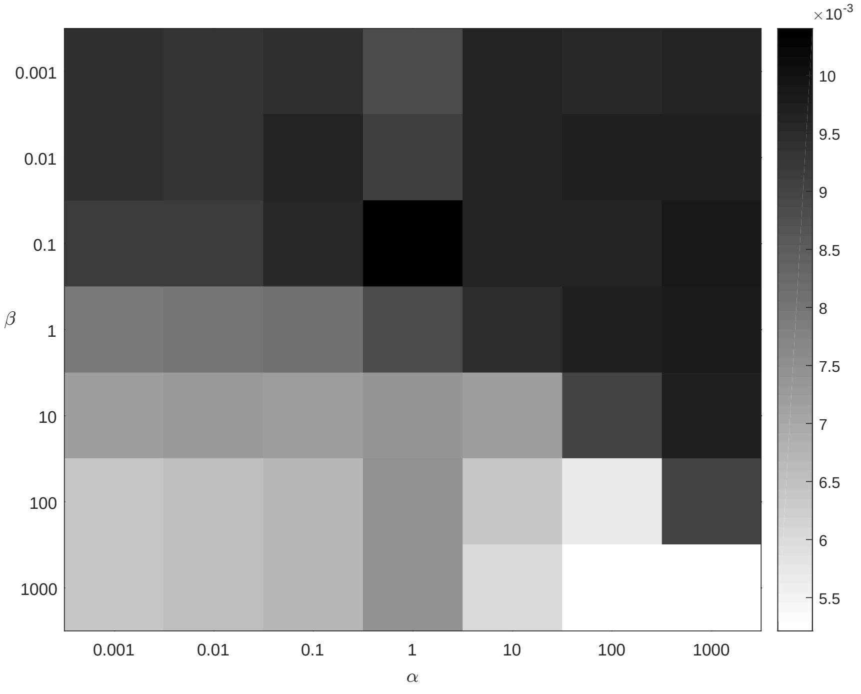


(b) Human PPI network was used as validation set

Figure 2: $F_1$ scores under different $\alpha$ and $\beta$ combinations
